# Supplementary material for: Breaking the Mold: Nonlinear Ranking Function Synthesis Without Templates
Source: arXiv:2409.18063 source file (2024-09-26)
Supplement: Supplementary file 1 [file appendix.tex]

\newpage

\appendix

\section{Proofs}

\printProofs
